# Supplementary material for: A forced thermal ratchet in a memory heat bath
Source: arXiv:2212.06333 source file (2022-12-13)
Supplement: Supplementary file 1 [file Appendix.tex]

\chapter{Cálculo del flujo de corriente en el caso Markoviano }
